# Supplementary material for: Empirical Security and Privacy Analysis of Mobile Symptom Checking Applications on Google Play
Source: arXiv:2107.13754 source file (2021-07-29)
Supplement: Supplementary file 1 [file appendix_long.tex]

\begin{table*}
  \caption{List of Symptom Checker Apps}
  \label{tab:apps_list}
  \scalebox{0.85} {
  \begin{tabular}{llrrrrll}
    \hline
    \hline
        {\bf No.} & {\bf Apps Name}  & {\bf \# of Installs} & {\bf Av. Rating} & {\bf Rated by} & {\bf \# of Review}  & {\bf Free} & {\bf \# of APK}\\ 
    \hline
        1 & com.webmd.android & 10,000,000+ & 4.44 & 64152 & 13448 & True & Single\\ 
        2 & com.ada.app & 5,000,000+ & 4.74 & 290484 & 133325 & True & Single\\ 
        3 & md.your & 1,000,000+ & 4.1 & 13981 & 3475 & True & Single\\ 
        4 & com.mayoclinic.patient & 1,000,000+ & 3.9 & 7642 & 3244 & True & Single\\ 
        
        % 5 & au.gov.health.covid19 & 500,000+ & 3.57 & 1621 & 801 & True & Single\\ 
        5 & com.programming.progressive.diagnoseapp & 500,000+ & 4.52 & 6276 & 2721 & True & Single\\ 
        6 & com.symptomate.mobile & 100,000+ & 4.41 & 2631 & 719 & True & Single\\ 
        7 & nl.japps.android.depressiontest & 100,000+ & 3.82 & 1535 & 464 & True & Single\\ 
        % 9 & symptoms.diary.tracker & 100,000+ & 4.09 & 1777 & 663 & False & Single\\ 
        8 & air.com.sensely.asknhs & 100,000+ & 4.29 & 2593 & 1197 & True & Single\\ 
        9 & com.caidr & 100,000+ & 4.08 & 505 & 286 & True & Single\\ 
        10 & com.teckelmedical.mediktor & 50,000+ & 3.62 & 1001 & 187 & True & Single\\ 
        11 & au.org.healthdirect.healthdirectapp & 50,000+ & 3.88 & 131 & 66 & True & Single\\ 
        12 & ai.mayamd.mayamd & 50,000+ & 4.3 & 121 & 40 & True & Single\\ 
        13 & de.msmix.foody.android & 10,000+ & 4.11 & 152 & 111 & True & Single\\ 
        14 & dk.kalorieopslag.symdir & 10,000+ & 3.39 & 124 & 77 & True & Single\\ 
        15 & com.appcolliders.doctordiagnose & 10,000+ & 3.5 & 130 & 27 & True & Single\\ 
        16 & com.epainassist.symptomchecker & 10,000+ & 3.28 & 50 & 18 & True & Single\\ 
        17 & baycare.com.healthnav & 10,000+ & 4.18 & 100 & 33 & True & Single\\ 
        18 & com.app.babycheck & 10,000+ & 3.03 & 31 & 22 & True & Single\\ 
        19 & com.bluecreate.vitamincheck & 10,000+ & 4.42 & 83 & 51 & True & Multiple\\ 
        20 & ai.tibot & 10,000+ & 3.74 & 170 & 105 & True & Single\\ 
        21 & andy.symptomes & 10,000+ & 3.79 & 155 & 62 & True & Single\\ 
        22 & com.appstronautstudios.headachetracker & 5,000+ & 4.19 & 58 & 32 & True & Single\\ 
        23 & com.app.diagnose & 5,000+ & 2.8 & 35 & 15 & True & Single\\ 
        24 & com.ro.doctor31 & 5,000+ & 3.69 & 105 & 59 & True & Single\\ 
        25 & com.worthyworks.multihtml & 1,000+ & 4.55 & 22 & 19 & True & Single\\ 
        26 & com.sylextech.youshieldapp & 1,000+ & 4.09 & 11 & 7 & True & Single\\ 
        27 & developer007.magdy.symptomchecker & 1,000+ & 0.0 & None & 0 & True & Multiple\\ 
        29 & com.pharma.mydiagnosis & 1,000+ & 3.88 & 8 & 5 & True & Single\\ 
        30 & com.prembros.symptomator & 1,000+ & 3.64 & 11 & 6 & True & Single\\ 
        31 & com.myownmed.quinnipiac & 500+ & 0.0 & None & 0 & True & Single\\ 
        32 & com.francotiveron.SymptomsChecker & 500+ & 0.0 & None & 0 & True & Single\\ 
        33 & com.worthyworks.myapplication & 500+ & 3.5 & 8 & 6 & True & Multiple\\ 
        34 & com.dietchartapp.medweiser & 100+ & 3.67 & 6 & 2 & True & Single\\ 
        35 & com.nextgenblue.symptomchecker & 100+ & 0.0 & None & 0 & True & Multiple\\ 
        36 & com.socmedica.symptomchecker & 50+ & 0.0 & None & 0 & True & Single\\ 
        37 & de.pr2.ebmapp & 10+ & 0.0 & None & 0 & True & Single\\     
\hline\hline
  \end{tabular}
  }
\end{table*}

\begin{table*}
  \caption{Result of apkid analysis}
  \label{tab:apps_list}
  \scalebox{0.850} {
  \begin{tabular}{rccccc}
    \hline\hline
    {\bf APK ID}  & {\bf Manipulator} & {\bf Anti-vm} & {\bf Anti-debug} & {\bf Anti-disassembly} & {\bf Obfuscator} \\    
    \hline
        air.com.sensely.asknhs & 0 & 1 & 1 & 0 & 0\\ 
        com.dietchartapp.medweiser & 0 & 0 & 0 & 0 & 0\\ 
        ai.mayamd.mayamd & 0 & 1 & 1 & 0 & 0\\ 
        ai.tibot & 0 & 1 & 1 & 1 & 0\\ 
        com.sylextech.youshieldapp & 1 & 1 & 0 & 0 & 0\\ 
        com.prembros.symptomator & 1 & 0 & 0 & 0 & 0\\ 
        andy.symptomes & 1 & 1 & 0 & 0 & 0\\ 
        com.worthyworks.myapplication & 0 & 1 & 0 & 0 & 0\\ 
        com.nextgenblue.symptomchecker& 0 & 1 & 1 & 0 & 0\\ 
        au.org.healthdirect.healthdirectapp & 0 & 1 & 1 & 0 & 0\\ 
        com.caidr & 0 & 1 & 1 & 0 & 0\\ 
        com.webmd.android & 0 & 1 & 1 & 0 & 0\\ 
        dk.kalorieopslag.symdir & 1 & 1 & 1 & 0 & 0\\ 
        com.app.babycheck & 0 & 1 & 1 & 0 & 0\\ 
        nl.japps.android.depressiontest & 1 & 1 & 0 & 0 & 0\\ 
        com.francotiveron.SymptomsChecker & 0 & 0 & 0 & 0 & 0\\ 
        com.myownmed.quinnipiac & 1 & 1 & 0 & 0 & 0\\ 
        com.pharma.mydiagnosis & 0 & 1 & 1 & 0 & 0\\ 
        com.appstronautstudios.headachetracker & 0 & 1 & 0 & 1 & 0\\ 
        md.your & 0 & 1 & 1 & 0 & 1\\ 
        com.bluecreate.vitamincheck & 0 & 1 & 1 & 0 & 0\\ 
        com.epainassist.symptomchecker & 1 & 1 & 1 & 0 & 0\\ 
        com.programming.progressive.diagnoseapp & 0 & 1 & 0 & 0 & 0\\ 
        de.pr2.ebmapp & 1 & 0 & 0 & 0 & 0\\ 
        com.ro.doctor31 & 0 & 1 & 1 & 0 & 0\\ 
        baycare.com.healthnav & 0 & 1 & 1 & 0 & 0\\ 
        com.app.diagnose & 0 & 1 & 1 & 0 & 0\\ 
        com.ada.app& 0 & 1 & 0 & 0 & 0\\ 
        com.mayoclinic.patient & 0 & 1 & 0 & 1 & 1\\ 
        de.msmix.foody.android & 0 & 1 & 1 & 0 & 0\\ 
        com.appcolliders.doctordiagnose & 0 & 1 & 0 & 0 & 0\\ 
        com.socmedica.symptomchecker & 0 & 1 & 0 & 0 & 0\\ 
        developer007.magdy.symptomchecker & 0 & 1 & 0 & 0 & 0\\ 
        com.symptomate.mobile & 0 & 1 & 0 & 0 & 0\\ 
        com.teckelmedical.mediktor & 0 & 1 & 1 & 0 & 0\\ 
        au.gov.health.covid19 & 0 & 1 & 1 & 0 & 0\\ 
        com.worthyworks.multihtml & 0 & 1 & 0 & 0 & 0\\ 
   \hline\hline
  \end{tabular}
  }
\end{table*}

\begin{table*}
  \caption{Permission Group by Level and Type}
  \label{tab:apps_list}
  \centering
  \scalebox{0.70} {
  \begin{tabular}{lll}
    \hline\hline
    Permission Type & Level & Count \\
    % \endhead
    \hline
    INTERNET & dangerous & 32\\ 
    ACCESS\_NETWORK\_STATE & normal & 29\\ 
    RECORD\_AUDIO & dangerous & 9\\ 
    READ\_EXTERNAL\_STORAGE & dangerous & 13\\ 
    WRITE\_EXTERNAL\_STORAGE & dangerous & 22\\ 
    CAMERA & dangerous & 12\\ 
    WAKE\_LOCK & dangerous & 19\\ 
    MODIFY\_AUDIO\_SETTINGS & dangerous & 7\\ 
    READ\_PHONE\_STATE & dangerous & 9\\ 
    CALL\_PHONE & dangerous & 6\\ 
    ACCESS\_COARSE\_LOCATION & dangerous & 11\\ 
    ACCESS\_FINE\_LOCATION & dangerous & 14\\ 
    BLUETOOTH & dangerous & 3\\ 
    RECEIVE & signature & 19\\ 
    BIND\_GET\_INSTALL\_REFERRER\_SERVICE & dangerous & 14\\ 
    BROADCAST\_STICKY & normal & 1\\ 
    C2D\_MESSAGE & signature & 10\\ 
    SYSTEM\_ALERT\_WINDOW & dangerous & 5\\ 
    MANAGE\_DOCUMENTS & signature & 3\\ 
    READ\_INTERNAL\_STORAGE & dangerous & 4\\ 
    USE\_FINGERPRINT & normal & 6\\ 
    VIBRATE & normal & 8\\ 
    INSTALL\_SHORTCUT & normal & 3\\ 
    READ\_CONTACTS & dangerous & 3\\ 
    READ\_CALENDAR & dangerous & 3\\ 
    WRITE\_CALENDAR & dangerous & 3\\ 
    WRITE\_SETTINGS & dangerous & 11\\ 
    ACCESS\_WIFI\_STATE & normal & 11\\ 
    RECEIVE\_BOOT\_COMPLETED & normal & 9\\ 
    REQUEST\_INSTALL\_PACKAGES & dangerous & 3\\ 
    STORAGE & dangerous & 3\\ 
    FOREGROUND\_SERVICE & normal & 6\\ 
    USE\_BIOMETRIC & normal & 4\\ 
    READ & dangerous & 6\\ 
    WRITE & dangerous & 6\\ 
    READ\_SETTINGS & dangerous & 14\\ 
    UPDATE\_SHORTCUT & dangerous & 6\\ 
    BROADCAST\_BADGE & dangerous & 6\\ 
    UPDATE\_COUNT & dangerous & 6\\ 
    UPDATE\_BADGE & dangerous & 6\\ 
    READ\_GSERVICES & dangerous & 7\\ 
    ACTIVITY\_RECOGNITION & dangerous & 4\\ 
    GET\_ACCOUNTS & normal & 3\\ 
    BILLING & dangerous & 6\\ 
    MAPS\_RECEIVE & dangerous & 1\\ 
    PROVIDER\_INSERT\_BADGE & dangerous & 4\\ 
    CHANGE\_BADGE & dangerous & 4\\ 
    READ\_APP\_BADGE & dangerous & 4\\ 
    BADGE\_COUNT\_READ & dangerous & 4\\ 
    BADGE\_COUNT\_WRITE & dangerous & 4\\ 
    WRITE\_CONTACTS & dangerous & 1\\ 
    GET\_TASKS & dangerous & 2\\ 
    SET\_ALARM & normal & 1\\ 
    WRITE\_INTERNAL\_STORAGE & dangerous & 2\\ 
    REQUEST\_IGNORE\_BATTERY\_OPTIMIZATIONS & normal & 1\\ 
    RECEIVE\_ADM\_MESSAGE & dangerous & 1\\ 
    USE\_CREDENTIALS & dangerous & 1\\ 
    READ\_PROFILE & dangerous & 1\\ 
    BODY\_SENSORS & dangerous & 2\\ 
    CHANGE\_WIFI\_MULTICAST\_STATE & dangerous & 1\\ 
    ACCESS\_NOTIFICATION\_POLICY & normal & 1\\ 
    CHECK\_LICENSE & dangerous & 1\\ 
    ACCESS\_BACKGROUND\_LOCATION & dangerous & 1\\ 
    BLUETOOTH\_ADMIN & dangerous & 1\\ 
    CHANGE\_WIFI\_STATE & dangerous & 1\\ 
    DISABLE\_KEYGUARD & dangerous & 1\\ 
    AUDIO & dangerous & 1\\     
    \hline\hline
  \end{tabular}
  }
\end{table*}

\begin{table*}
  \caption{Certificate Signing Analysis}
  \label{tab:apps_list}
  \centering
  \scalebox{0.85} {
  \begin{tabular}{lll}
    \hline\hline
        Apps Name  &  Signature Algorithm & Key Length \\     
    % \endhead
    \hline
        com.myownmed.quinnipiac.apk &  SHA256 + RSA &  2048\\ 
        com.appcolliders.doctordiagnose.apk &  SHA256 + RSA &  2048\\ 
        nl.japps.android.depressiontest.apk &  SHA1 + RSA (weak) &  2048\\ 
        com.ro.doctor31.apk &  SHA256 + RSA &  4096\\ 
        com.dietchartapp.medweiser.apk &  SHA256 + RSA &  4096\\ 
        com.francotiveron.SymptomsChecker.apk &  SHA256 + RSA &  4096\\ 
        com.socmedica.symptomchecker.apk &  SHA256 + RSA &  4096\\ 
        com.teckelmedical.mediktor.apk &  SHA256 + RSA &  2048\\ 
        dk.kalorieopslag.symdir.apk &  SHA256 + RSA &  2048\\ 
        ai.mayamd.mayamd.apk &  SHA256 + RSA &  4096\\ 
        com.mayoclinic.patient.apk &  SHA1 + RSA (weak) &  2048\\ 
        com.worthyworks.myapplication.apk &  SHA256 + RSA &  4096\\ 
        md.your.apk &  SHA256 + RSA &  2048\\ 
        com.bluecreate.vitamincheck.apk &  SHA256 + RSA &  4096\\ 
        com.nextgenblue.symptomchecker.apk &  SHA256 + RSA &  4096\\ 
        developer007.magdy.symptomchecker.apk &  SHA256 + RSA &  4096\\ 
        com.webmd.android.apk &  SHA1 + RSA (weak) &  2048\\ 
        andy.symptomes.apk &  SHA256 + RSA &  2048\\ 
        com.sylextech.youshieldapp.apk &  SHA256 + RSA &  2048\\ 
        air.com.sensely.asknhs.apk & SHA1 + RSA (weak) &  2048\\
        de.msmix.foody.android.apk &  SHA256 + RSA &  2048\\ 
        com.programming.progressive.diagnoseapp.apk &  SHA256 + RSA &  2048\\ 
        baycare.com.healthnav.apk &  SHA256 + RSA &  2048\\ 
        com.ada.app.apk &  SHA256 + RSA &  2048\\ 
        com.app.diagnose.apk &  SHA256 + RSA &  4096\\ 
        de.pr2.ebmapp.apk &  SHA256 + RSA &  4096\\ 
        com.appstronautstudios.headachetracker.apk &  SHA256 + RSA &  4096\\ 
        com.symptomate.mobile.apk &  SHA1 + RSA (weak) &  2048\\ 
        com.worthyworks.multihtml.apk &  SHA256 + RSA &  4096\\ 
        com.epainassist.symptomchecker.apk &  SHA256 + RSA &  2048\\ 
        ai.tibot.apk &  SHA256 + RSA &  4096\\ 
        com.prembros.symptomator.apk &  SHA256 + RSA &  2048\\ 
        com.pharma.mydiagnosis.apk &  SHA256 + RSA &  2048\\ 
        au.org.healthdirect.healthdirectapp.apk &  SHA256 + RSA &  2048\\ 
        com.caidr.apk &  SHA256 + RSA &  2048\\ 
        com.app.babycheck.apk &  SHA256 + RSA &  4096\\ 
    \hline\hline
  \end{tabular}
  }
\end{table*}

\begin{table*}
  \caption{Exported Component Analysis. \ik{remove .apk from the app ids.}}
  \label{tab:exported_component}
  \centering
  \scalebox{0.85} {
  \begin{tabular}{lllll}
    \hline
        File Name & Exported Activities & Exported Services & Exported Receiver & Exported Provider.  \\ 
            % \endhead
    \hline\hline
        com.webmd.android.apk & 12 & 1 & 4 & 0\\ 
        ai.mayamd.mayamd.apk & 10 & 2 & 6 & 0\\ 
        com.socmedica.symptomchecker.apk & 10 & 2 & 6 & 0\\ 
        com.caidr.apk & 8 & 2 & 6 & 0\\ 
        com.bluecreate.vitamincheck_cp.apk & 8 & 2 & 6 & 0\\ 
        ai.tibot.apk & 4 & 2 & 3 & 0\\ 
        com.prembros.symptomator.apk & 4 & 0 & 0 & 0\\ 
        md.your.apk & 4 & 3 & 5 & 0\\ 
        com.mayoclinic.patient.apk & 4 & 5 & 3 & 0\\ 
        au.org.healthdirect.healthdirectapp.apk & 2 & 1 & 5 & 0\\ 
        com.app.diagnose.apk & 2 & 2 & 2 & 0\\ 
        com.appcolliders.doctordiagnose.apk & 2 & 0 & 0 & 0\\ 
        com.nextgenblue.symptomchecker_cp.apk & 1 & 4 & 3 & 0\\ 
        com.appstronautstudios.headachetracker.apk & 1 & 2 & 3 & 0\\ 
        baycare.com.healthnav.apk & 1 & 1 & 2 & 0\\ 
        com.teckelmedical.mediktor.apk & 1 & 3 & 3 & 0\\ 
        air.com.sensely.asknhs.apk & 0 & 1 & 1 & 0\\ 
        com.dietchartapp.medweiser.apk & 0 & 0 & 0 & 0\\ 
        com.sylextech.youshieldapp.apk & 0 & 0 & 0 & 0\\ 
        andy.symptomes.apk & 0 & 1 & 0 & 0\\ 
        com.worthyworks.myapplication_cp.apk & 0 & 1 & 1 & 0\\ 
        dk.kalorieopslag.symdir.apk & 0 & 0 & 0 & 0\\ 
        com.app.babycheck.apk & 0 & 0 & 0 & 0\\ 
        l.japps.android.depressiontest.apk & 0 & 1 & 3 & 0\\ 
        com.francotiveron.SymptomsChecker.apk & 0 & 0 & 0 & 0\\ 
        com.myownmed.quinnipiac.apk & 0 & 3 & 2 & 0\\ 
        com.pharma.mydiagnosis.apk & 0 & 2 & 6 & 0\\ 
        com.epainassist.symptomchecker.apk & 0 & 0 & 1 & 0\\ 
        com.programming.progressive.diagnoseapp.apk & 0 & 0 & 0 & 0\\ 
        de.pr2.ebmapp.apk & 0 & 0 & 0 & 0\\ 
        com.ro.doctor31.apk & 0 & 0 & 1 & 0\\ 
        com.ada.app.apk & 0 & 0 & 3 & 0\\ 
        de.msmix.foody.android.apk & 0 & 0 & 1 & 0\\ 
        developer007.magdy.symptomchecker_cp.apk & 0 & 0 & 0 & 0\\ 
        com.symptomate.mobile.apk & 0 & 1 & 0 & 0\\ 
        com.worthyworks.multihtml.apk & 0 & 0 & 0 & 0\\     
    \hline\hline
  \end{tabular}
  }
\end{table*}

\begin{table*}
  \caption{Number of Tracker per Apps}
  \label{tab:exported_component}
  \centering
  \scalebox{0.90} {
  \begin{tabular}{llr}
    \hline\hline
        No & Apps Name & Number of Tracker \\ 
            % \endhead
    \hline
        1 & com.caidr.apk & 10\\
        2 & ai.mayamd.mayamd.apk & 9\\
        3 & com.webmd.android.apk & 9\\
        4 & com.teckelmedical.mediktor.apk & 9\\
        5 & baycare.com.healthnav.apk & 8\\
        6 & com.socmedica.symptomchecker.apk & 8\\
        7 & ai.tibot.apk & 8\\
        8 & md.your.apk & 6\\
        9 & au.org.healthdirect.healthdirectapp.apk & 5\\
        10 & com.ada.app.apk & 4\\
        11 & dk.kalorieopslag.symdir.apk & 3\\
        12 & com.appstronautstudios.headachetracker.apk & 3\\
        13 & com.myownmed.quinnipiac.apk & 3\\
        14 & com.programming.progressive.diagnoseapp.apk & 2\\
        15 & com.worthyworks.multihtml.apk & 2\\
        16 & nl.japps.android.depressiontest.apk & 2\\
        17 & com.pharma.mydiagnosis.apk & 2\\
        18 & com.app.diagnose.apk & 2\\
        20 & air.com.sensely.asknhs.apk & 2\\
        21 & com.ro.doctor31.apk & 1\\
        22 & com.appcolliders.doctordiagnose.apk & 1\\
        23 & com.app.babycheck.apk & 1\\
        24 & de.msmix.foody.android.apk & 1\\
        25 & andy.symptomes.apk & 1\\
        26 & com.mayoclinic.patient.apk & 1\\    
    \hline\hline
  \end{tabular}
  }
\end{table*}

\begin{table*}
  \caption{Number Unique URL connection using HTTP or HTTPS. \ik{Remove .har from the apps ids.}}
  \label{tab:http_https}
  \centering
  \scalebox{0.85} {
  \begin{tabular}{llr}
    \hline\hline
        App Name & HTTP & HTTPS \\ 
            % \endhead
    \hline
        air.com.sensely.asknhs.har & 2 & 109\\ 
        com.francotiveron.SymptomsChecker.har & 3 & 35\\ 
        com.app.babycheck.har & 2 & 68\\ 
        nl.japps.android.depressiontest.har & 1 & 28\\ 
        com.app.diagnose.har & 1 & 70\\ 
        com.teckelmedical.mediktor.har & 1 & 47\\ 
        andy.symptomes.har & 1 & 3\\ 
        com.epainassist.symptomchecker.har & 1 & 97\\ 
        com.pharma.mydiagnosis.har & 3 & 20\\ 
        com.appstronautstudios.headachetracker.har & 1 & 7\\ 
        com.worthyworks.multihtml.har & 3 & 118\\ 
        au.org.healthdirect.healthdirectapp.har & 2 & 91\\ 
        de.pr2.ebmapp.har & 26 & 30\\ 
        ai.tibot.har & 3 & 95\\ 
        com.mayoclinic.patient.har & 2 & 93\\ 
        dk.kalorieopslag.symdir.har & 2 & 3\\ 
        com.ro.doctor31.har & 1 & 7\\ 
        com.caidr.har & 1 & 51\\ 
        com.symptomate.mobile.har & 1 & 66\\ 
        com.sylextech.youshieldapp.har & 3 & 12\\ 
        com.prembros.symptomator.har & 1 & 2\\ 
        ai.mayamd.mayamd.har & 1 & 30\\ 
        md.your.har & 2 & 37\\ 
        de.msmix.foody.android.har & 3 & 5\\ 
        com.ada.app.har & 1 & 27\\ 
        com.socmedica.symptomchecker.har & 1 & 9\\ 
        com.dietchartapp.medweiser.har & 1 & 307\\ 
        baycare.com.healthnav.har & 3 & 35\\ 
        com.programming.progressive.diagnoseapp.har & 1 & 3\\ 
        com.appcolliders.doctordiagnose.har & 0 & 5\\ 
    \hline\hline
  \end{tabular}
  
  }
\end{table*}

\begin{table*}
  \caption{Number of URL Connection to First or Third Party}
  \label{tab:first_third}
  \centering
  \scalebox{0.85} {
  \begin{tabular}{llr}
    \hline\hline
        App Name & First & Third \\ 
            % \endhead
    \hline
        air.com.sensely.asknhs.har & 104 & 7\\ 
        com.francotiveron.SymptomsChecker.har & 38 & 0\\ 
        com.app.babycheck.har & 57 & 13\\ 
        nl.japps.android.depressiontest.har & 25 & 4\\ 
        com.app.diagnose.har & 55 & 16\\ 
        com.teckelmedical.mediktor.har & 41 & 7\\ 
        andy.symptomes.har & 1 & 3\\ 
        com.epainassist.symptomchecker.har & 95 & 3\\ 
        com.pharma.mydiagnosis.har & 20 & 3\\ 
        com.appstronautstudios.headachetracker.har & 1 & 7\\ 
        com.worthyworks.multihtml.har & 110 & 11\\ 
        au.org.healthdirect.healthdirectapp.har & 64 & 29\\ 
        de.pr2.ebmapp.har & 52 & 4\\ 
        ai.tibot.har & 53 & 45\\ 
        com.mayoclinic.patient.har & 94 & 1\\ 
        dk.kalorieopslag.symdir.har & 2 & 3\\ 
        com.ro.doctor31.har & 5 & 3\\ 
        com.caidr.har & 20 & 32\\ 
        com.symptomate.mobile.har & 34 & 33\\ 
        com.sylextech.youshieldapp.har & 3 & 12\\ 
        com.prembros.symptomator.har & 1 & 2\\ 
        ai.mayamd.mayamd.har & 31 & 0\\ 
        md.your.har & 28 & 11\\ 
        de.msmix.foody.android.har & 4 & 4\\ 
        com.ada.app.har & 20 & 8\\ 
        com.socmedica.symptomchecker.har & 10 & 0\\ 
        com.dietchartapp.medweiser.har & 292 & 16\\ 
        baycare.com.healthnav.har & 19 & 19\\ 
        com.programming.progressive.diagnoseapp.har & 1 & 3\\ 
        com.appcolliders.doctordiagnose.har & 3 & 2\\ 
    \hline\hline
  \end{tabular}
  }
\end{table*}

\section{User complaint categories}
\label{app:complaints}

%Table~\ref{tab:complaintallcat} reports the different complaint  categories defined for the analysis of negative mHealth app reviews, and the corresponding sets of case-insensitive keywords searched in the app reviews' texts.

\begin{table*}[h]
\caption{Complaint categories defined for the app review analysis. \label{tab:complaintallcat}}
\label{cat:complaint_categories}
\small
\centering
%\resizebox{\linewidth}{!}
{%
\begin{tabular}{l | p{10cm}  }
\hline\hline
\textbf{Complaint category} & \textbf{Case-insensitive keywords} \\
\hline
\hline
\textit{Usability:} & \\
Bugs & force close; crash; bug; freeze; glitch; froze; stuck; stick; error; disconnect; not work; not working \\
Battery & battery; cpu; processor; processing;  ram ; memory\\
Mobile Data & mobile data; gb; mb; background data; \\  \midrule
\hline
\textit{Mal-behaviour:} & \\
Scam & scam; credit card; bad business; bad app\\
Adult & porn; adult; adult ad\\
Offensive; Hate & sexis; LGBT; trolling; racism; offensive; islamophobia; vile word; minorities; hate speech; shit storm\\ \hline
\hline
\textit{Privacy:} & \\
Privacy & privacy; private; personal details; personal info; personal data\\
Ads & ads; ad; advertisement; advertising; intrusive; annoying ad; popup; inappropriate; video ads; in-app ads\\
Trackers & tracker; track; tracking\\ \midrule
\hline
\textit{Security:} & \\
Security & security; tls; certificate; attack\\
Malware & malware; trojan; adware; phishing; suspicious; malicious; spyware \\
Intrusive Permissions & permission\\

\hline\hline

% \hhline{=====}
\end{tabular}
}
\end{table*}
% \subsection{Part One}
